# Supplementary material for: Sparseloop: An Analytical Approach To Sparse Tensor Accelerator Modeling
Source: arXiv:2205.05826 source file (2023-01-09)
Supplement: Supplementary file 1 [file 09_revision_appendix.tex]

\section{Revision Appendix}
This revision includes the following major modifications (highlighted in red in the original content)
\begin{itemize}

    \item \textbf{Section~\ref{sec:exp_val} Validation Against Real Hardware}
    \begin{itemize}
        \item \textbf{Reviewer C suggested clarifying the motivation for using old/different workloads for existing design validations}. We further clarified the reasons for using different workloads for different accelerator's validation in the \underline{Section~\ref{sec:exp_val} prologue}, but basically we were limited to what was available for those designs.
        \item \textbf{Reviewer C, E both ask for more details on validation, and were in particularly interested in validation against real hardware} We added validation against real hardware, \ie, NVIDIA's sparse tensor core in \underline{Section~\ref{sec:stc}} and clarification of baseline setups for the accelerators from research proposals to indicate whether real hardware is used in \underline{Section~\ref{sec:exp_val} prologue}, \underline{Table~\ref{tab:validation_summary}}, \underline{Section~\ref{sec:dstc}}, and \\ \underline{Section~\ref{sec:eyeriss}}.
        \item \textbf{Reviewer C asks for validation on NVDLA with sparse weights}.  Modeling sparse weights with NV Xavier entails specification of the compression SAF, which is the only SAF embodied in NVDLA. We are highly confident that SparseTile would accurately model the NVDLA accelerator due to i)  the pre-existing validation of Timeloop-ISPASS19 to model NVDLA without compression; ii) our ability to  model compression SAFs for Eyeriss and Eyeriss V2, which are similar to what NVDLA uses. Since specifying/validating the sparse NVDLA would require more time than is available in the revision time frame,  as a surrogate for that design we added a more detailed validation on Eyeriss' DRAM compression SAF in \underline{Section~\ref{sec:eyeriss}  and Table~\ref{tab:v1_compression}}. 
        \item \textbf{Reviewer A suggested we  demonstrate \tool's ability to model the structured sparsity supported by the Ampere GPU's sparse tensor core}: We added a new validation for Ampere's sparse tensor core in \underline{Section~\ref{sec:stc}}.
        
    \end{itemize}
    \item \textbf{Section~\ref{sec:stc-study} Strong Use Case: Investigating Next Generation Sparse Tensor Core with \tool}
        \begin{itemize}
        \item \textbf{Reviewer A, B, D suggested including a strong use case of \tool~to demonstrate its applications in 1) comparing various designs (especially comparisons related to sparse tensor core in GPU) and 2) usage in an example design flow for developing new accelerators }: We replaced the original case study with an easier to understand and stronger use case of \tool~in an accelerator design flow for i) performing an apples-to-apples comparison of two accelerators: the Ampere GPU's sparse tensor core~\cite{ampere-white-paper} and the dual side sparse tensor core~\cite{dual-side-tensor-core}; ii) identifying limitations of the current sparse tensor core architecture; iii) finding possible solutions to designing a next generation sparse tensor core. 
    \end{itemize}
    
    \item \textbf{Section~\ref{sec:speed} Simulation Speed} 
    \begin{itemize}
        \item \textbf{Reviewer D suggested providing more information to justify the 2000$\times$ speedup of \tool.} We included more details on the reasons for \tool's fast modeling speed compared to cycle-level simulations, basically that an analytical model can extrapolate what happens in many cycles without simulating each one.
    \end{itemize}
    \item \textbf{Abstract, Introduction, Conclusion}: patches to reflect body section changes.
\end{itemize}
